# Supplementary material for: Prediction of interesting ferromagnetism in Janus semiconducting Cr$_2$AsP monolayer
Source: arXiv:2210.13727 source file (2023-04-10)
Supplement: Supplementary file 1 [file Supplemental_Material.pdf]

# Prediction of interesting ferromagnetism in Janus semiconducting $Cr_2AsP$ monolayer

Qiuyue Ma, Guochun Yang and Yong Liu*

State Key Laboratory of Metastable Materials Science and Technology & Key Laboratory for Microstructural Material Physics of Hebei Province, School of Science, Yanshan University, Qinhuangdao 066004, China

*Email: yongliu@ysu.edu.cn

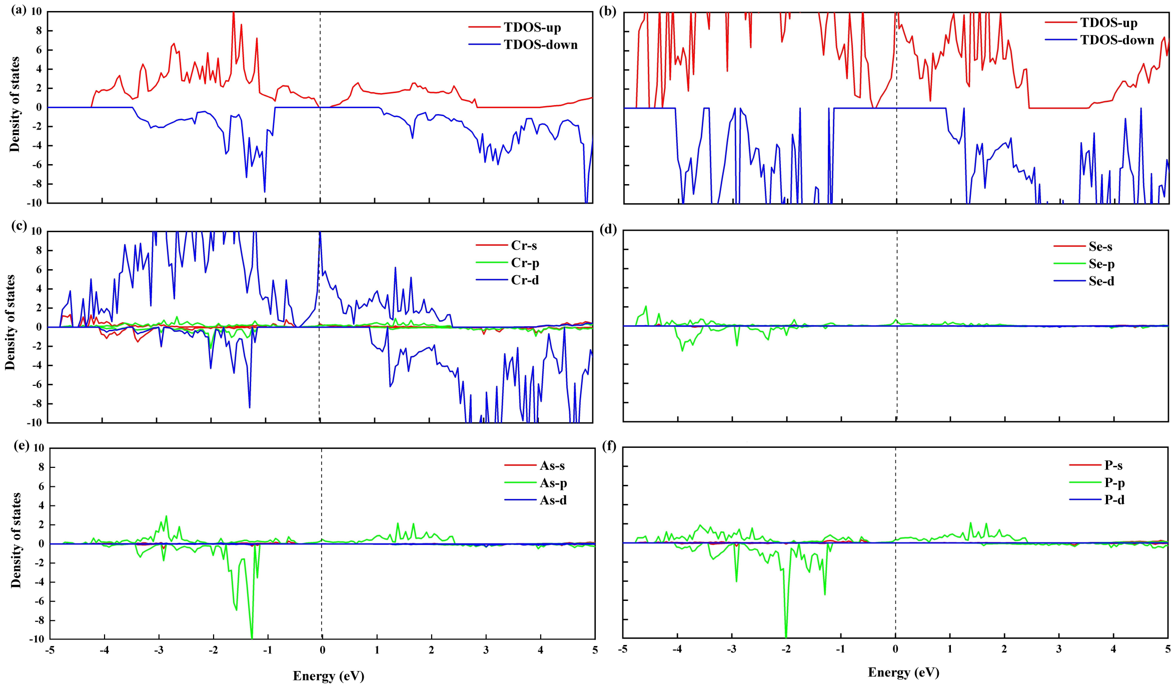


Fig.S1. Total density of states (TDOS) of (a) $Cr_2AsP$ and (b) $Cr_2As_{0.25}Se_{0.75}P$ monolayers. (c)-(f) Projected density states (PDOS) of $Cr_2As_{0.25}Se_{0.75}P$ monolayer.

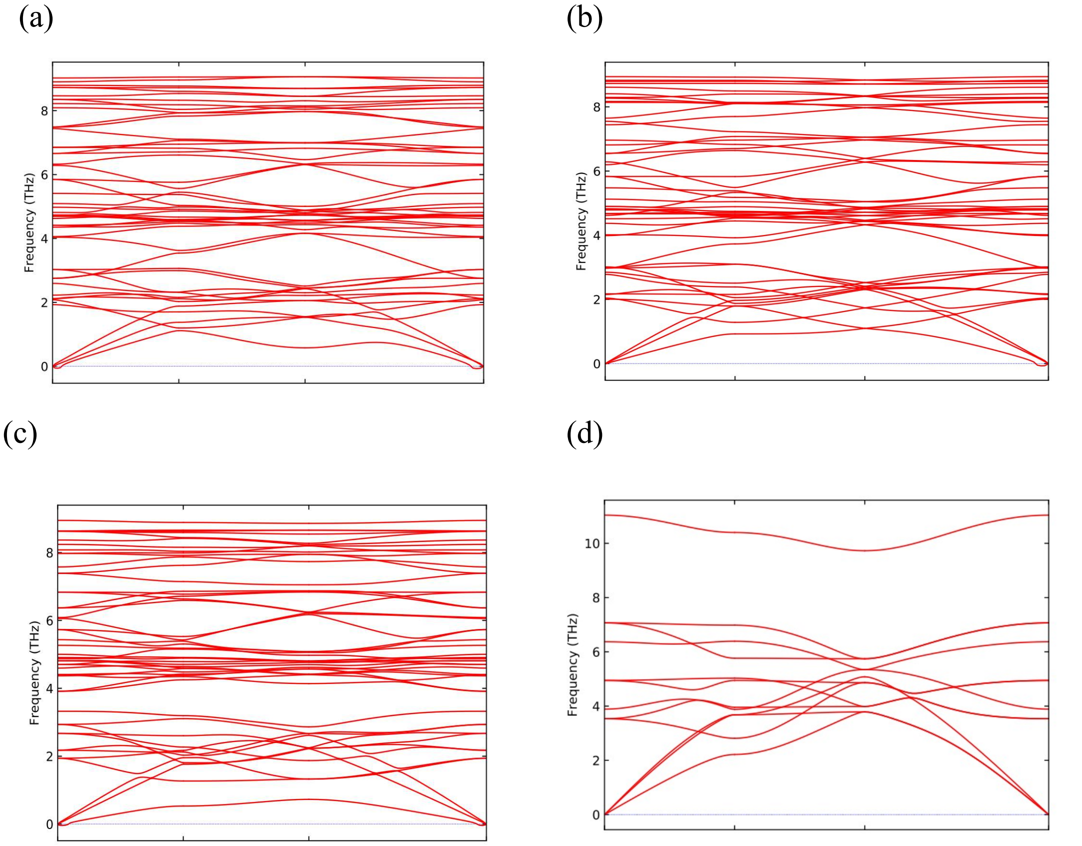


Fig.S2. Phonon spectrum of monolayer (a) $Cr_2As_{0.25}Se_{0.75}P$, (b) $Cr_2As_{0.5}Se_{0.5}P$, (d) $Cr_2As_{0.75}Se_{0.25}P$, (d) $Cr_2SeP$
